# Supplementary material for: ForecastTKGQuestions: A Benchmark for Temporal Question Answering and Forecasting over Temporal Knowledge Graphs
Source: arXiv:2208.06501 source file (2023-07-18)
Supplement: Supplementary file 1 [file Technical_Appendix.pdf]

# FORECASTTKGQUESTIONS: A Benchmark for Temporal Question Answering and Forecasting over Temporal Knowledge Graphs

Anonymous submission

## Appendix

### A Scoring Function Details

#### A.1 Entity Prediction

The detailed definition of the entity prediction questions' scoring function is defined as

$$\begin{aligned}
 es(e) &= \text{Re}(\langle \mathbf{h}'_{(s,t_q)}, \mathbf{h}_q, \bar{\mathbf{h}}'_{(e,t_q)} \rangle) \\
 &= \text{Re} \left( \sum_{k=1}^d \mathbf{h}'_{(s,t_q)}(k) \cdot \mathbf{h}_q(k) \cdot \bar{\mathbf{h}}'_{(e,t_q)}(k) \right) \\
 &= \langle \text{Re}(\mathbf{h}'_{(s,t_q)}), \text{Re}(\mathbf{h}_q), \text{Re}(\mathbf{h}'_{(e,t_q)}) \rangle \\
 &\quad + \langle \text{Re}(\mathbf{h}'_{(s,t_q)}), \text{Im}(\mathbf{h}_q), \text{Im}(\mathbf{h}'_{(e,t_q)}) \rangle \\
 &\quad + \langle \text{Im}(\mathbf{h}'_{(s,t_q)}), \text{Re}(\mathbf{h}_q), \text{Im}(\mathbf{h}'_{(e,t_q)}) \rangle \\
 &\quad - \langle \text{Im}(\mathbf{h}'_{(s,t_q)}), \text{Im}(\mathbf{h}_q), \text{Re}(\mathbf{h}'_{(e,t_q)}) \rangle.
 \end{aligned} \tag{1}$$

Re and Im denote taking the real part and the imaginary part of the complex vector, respectively.  $\mathbf{h}'_{(s,t_q)}, \mathbf{h}_q, \mathbf{h}'_{(e,t_q)} \in \mathbb{C}^d$ .  $\mathbf{h}'_{(s,t_q)}(k)$  denotes the  $k$ th element of it (same for  $\mathbf{h}_q$  and  $\mathbf{h}'_{(e,t_q)}$ ).  $\langle \mathbf{v}_1, \mathbf{v}_2, \mathbf{v}_3 \rangle = \sum_{k=1}^d \mathbf{v}_1(k) \cdot \mathbf{v}_2(k) \cdot \mathbf{v}_3(k)$  denotes the dot product of three  $d$ -dimensional complex vectors  $\mathbf{v}_1, \mathbf{v}_2, \mathbf{v}_3 \in \mathbb{C}^d$ .

#### A.2 Yes-No

The detailed definition of the yes-no questions' scoring functions are defined as

$$\begin{aligned}
 ys &= \text{Re}(\langle \mathbf{h}'_{(s,t_q)}, \mathbf{h}_q, \bar{\mathbf{h}}'_{(o,t_q)}, \mathbf{h}_{\text{yes}} \rangle) \\
 &= \text{Re} \left( \sum_{k=1}^d \mathbf{h}'_{(s,t_q)}(k) \cdot \mathbf{h}_q(k) \cdot \bar{\mathbf{h}}'_{(o,t_q)}(k) \cdot \mathbf{h}_{\text{yes}}(k) \right) \\
 &= \langle \text{Re}(\mathbf{h}'_{(s,t_q)}), \text{Re}(\mathbf{h}_q), \text{Re}(\mathbf{h}'_{(o,t_q)}), \text{Re}(\mathbf{h}_{\text{yes}}) \rangle \\
 &\quad + \langle \text{Re}(\mathbf{h}'_{(s,t_q)}), \text{Im}(\mathbf{h}_q), \text{Im}(\mathbf{h}'_{(o,t_q)}), \text{Re}(\mathbf{h}_{\text{yes}}) \rangle \\
 &\quad + \langle \text{Im}(\mathbf{h}'_{(s,t_q)}), \text{Re}(\mathbf{h}_q), \text{Im}(\mathbf{h}'_{(o,t_q)}), \text{Re}(\mathbf{h}_{\text{yes}}) \rangle \\
 &\quad + \langle \text{Re}(\mathbf{h}'_{(s,t_q)}), \text{Re}(\mathbf{h}_q), \text{Im}(\mathbf{h}'_{(o,t_q)}), \text{Im}(\mathbf{h}_{\text{yes}}) \rangle \\
 &\quad - \langle \text{Im}(\mathbf{h}'_{(s,t_q)}), \text{Im}(\mathbf{h}_q), \text{Re}(\mathbf{h}'_{(o,t_q)}), \text{Re}(\mathbf{h}_{\text{yes}}) \rangle \\
 &\quad - \langle \text{Im}(\mathbf{h}'_{(s,t_q)}), \text{Re}(\mathbf{h}_q), \text{Re}(\mathbf{h}'_{(o,t_q)}), \text{Im}(\mathbf{h}_{\text{yes}}) \rangle \\
 &\quad - \langle \text{Im}(\mathbf{h}'_{(s,t_q)}), \text{Im}(\mathbf{h}_q), \text{Im}(\mathbf{h}'_{(o,t_q)}), \text{Im}(\mathbf{h}_{\text{yes}}) \rangle \\
 &\quad - \langle \text{Re}(\mathbf{h}'_{(s,t_q)}), \text{Im}(\mathbf{h}_q), \text{Re}(\mathbf{h}'_{(o,t_q)}), \text{Im}(\mathbf{h}_{\text{yes}}) \rangle.
 \end{aligned} \tag{2}$$

$$\begin{aligned}
 ns &= \text{Re}(\langle \mathbf{h}'_{(s,t_q)}, \mathbf{h}_q, \bar{\mathbf{h}}'_{(o,t_q)}, \mathbf{h}_{\text{no}} \rangle) \\
 &= \text{Re} \left( \sum_{k=1}^d \mathbf{h}'_{(s,t_q)}(k) \cdot \mathbf{h}_q(k) \cdot \bar{\mathbf{h}}'_{(o,t_q)}(k) \cdot \mathbf{h}_{\text{no}}(k) \right) \\
 &= \langle \text{Re}(\mathbf{h}'_{(s,t_q)}), \text{Re}(\mathbf{h}_q), \text{Re}(\mathbf{h}'_{(o,t_q)}), \text{Re}(\mathbf{h}_{\text{no}}) \rangle \\
 &\quad + \langle \text{Re}(\mathbf{h}'_{(s,t_q)}), \text{Im}(\mathbf{h}_q), \text{Im}(\mathbf{h}'_{(o,t_q)}), \text{Re}(\mathbf{h}_{\text{no}}) \rangle \\
 &\quad + \langle \text{Im}(\mathbf{h}'_{(s,t_q)}), \text{Re}(\mathbf{h}_q), \text{Im}(\mathbf{h}'_{(o,t_q)}), \text{Re}(\mathbf{h}_{\text{no}}) \rangle \\
 &\quad + \langle \text{Re}(\mathbf{h}'_{(s,t_q)}), \text{Re}(\mathbf{h}_q), \text{Im}(\mathbf{h}'_{(o,t_q)}), \text{Im}(\mathbf{h}_{\text{no}}) \rangle \\
 &\quad - \langle \text{Im}(\mathbf{h}'_{(s,t_q)}), \text{Im}(\mathbf{h}_q), \text{Re}(\mathbf{h}'_{(o,t_q)}), \text{Re}(\mathbf{h}_{\text{no}}) \rangle \\
 &\quad - \langle \text{Im}(\mathbf{h}'_{(s,t_q)}), \text{Re}(\mathbf{h}_q), \text{Re}(\mathbf{h}'_{(o,t_q)}), \text{Im}(\mathbf{h}_{\text{no}}) \rangle \\
 &\quad - \langle \text{Im}(\mathbf{h}'_{(s,t_q)}), \text{Im}(\mathbf{h}_q), \text{Im}(\mathbf{h}'_{(o,t_q)}), \text{Im}(\mathbf{h}_{\text{no}}) \rangle \\
 &\quad - \langle \text{Re}(\mathbf{h}'_{(s,t_q)}), \text{Im}(\mathbf{h}_q), \text{Re}(\mathbf{h}'_{(o,t_q)}), \text{Im}(\mathbf{h}_{\text{no}}) \rangle.
 \end{aligned} \tag{3}$$

#### A.3 Fact Reasoning

The detailed definition of fact reasoning questions' scoring function is defined as

$$\begin{aligned}
 cs(c_i) &= \text{Re}(\langle \mathbf{h}'_{(s_i,t_i)}, \mathbf{h}_q^{c_i}, \bar{\mathbf{h}}'_{(o_i,t_i)}, \mathbf{h}'_q \rangle) \\
 &= \text{Re} \left( \sum_{k=1}^d \mathbf{h}'_{(s_i,t_i)}(k) \cdot \mathbf{h}_q^{c_i}(k) \cdot \bar{\mathbf{h}}'_{(o_i,t_i)}(k) \cdot \mathbf{h}'_q(k) \right) \\
 &= \langle \text{Re}(\mathbf{h}'_{(s_i,t_i)}), \text{Re}(\mathbf{h}_q^{c_i}), \text{Re}(\mathbf{h}'_{(o_i,t_i)}), \text{Re}(\mathbf{h}'_q(k)) \rangle \\
 &\quad + \langle \text{Re}(\mathbf{h}'_{(s_i,t_i)}), \text{Im}(\mathbf{h}_q^{c_i}), \text{Im}(\mathbf{h}'_{(o_i,t_i)}), \text{Re}(\mathbf{h}'_q(k)) \rangle \\
 &\quad + \langle \text{Im}(\mathbf{h}'_{(s_i,t_i)}), \text{Re}(\mathbf{h}_q^{c_i}), \text{Im}(\mathbf{h}'_{(o_i,t_i)}), \text{Re}(\mathbf{h}'_q(k)) \rangle \\
 &\quad + \langle \text{Re}(\mathbf{h}'_{(s_i,t_i)}), \text{Re}(\mathbf{h}_q^{c_i}), \text{Im}(\mathbf{h}'_{(o_i,t_i)}), \text{Im}(\mathbf{h}'_q(k)) \rangle \\
 &\quad - \langle \text{Im}(\mathbf{h}'_{(s_i,t_i)}), \text{Im}(\mathbf{h}_q^{c_i}), \text{Re}(\mathbf{h}'_{(o_i,t_i)}), \text{Re}(\mathbf{h}'_q(k)) \rangle \\
 &\quad - \langle \text{Im}(\mathbf{h}'_{(s_i,t_i)}), \text{Re}(\mathbf{h}_q^{c_i}), \text{Re}(\mathbf{h}'_{(o_i,t_i)}), \text{Im}(\mathbf{h}'_q(k)) \rangle \\
 &\quad - \langle \text{Im}(\mathbf{h}'_{(s_i,t_i)}), \text{Im}(\mathbf{h}_q^{c_i}), \text{Im}(\mathbf{h}'_{(o_i,t_i)}), \text{Im}(\mathbf{h}'_q(k)) \rangle \\
 &\quad - \langle \text{Re}(\mathbf{h}'_{(s_i,t_i)}), \text{Im}(\mathbf{h}_q^{c_i}), \text{Re}(\mathbf{h}'_{(o_i,t_i)}), \text{Im}(\mathbf{h}'_q(k)) \rangle.
 \end{aligned} \tag{4}$$

## B Implementation Details

We implement all the experiments with PyTorch (Paszke et al. 2019) on an NVIDIA A40 with 48GB memory and a 2.6GHZ AMD EPYC 7513 32-Core Processor.

## B.1 Temporal Knowledge Graph Forecasting

We train TANGO and TComplEx to perform TKG forecasting on ICEWS21. We implement TANGO with the official implementation. We switch its scoring function to ComplEx and perform a grid search for the embedding size (the dimension  $d$  of the entity and relation representations). We keep the rest hyperparameters as its default setting of the ICEWS05-15 dataset. We train TComplEx with the official implementation. We perform a grid search for the embedding size and keep the other hyperparameters as their default values. Table 1 provides the searching spaces of the grid searches for both methods. For each method, we run TKG forecasting experiments with different embedding sizes and choose the setting that leads to the best validation MRR as the best hyperparameter setting. We further run TANGO + Tucker with the best hyperparameters searched with TANGO + ComplEx for studying the effectiveness of different TKG scoring functions.

| Embedding Size Search Space |                          |
|-----------------------------|--------------------------|
| TANGO                       | {50, <b>100</b> , 150}   |
| TComplEx                    | { <b>100</b> , 136, 174} |

Table 1: Embedding size search space of TANGO and TComplEx. The embedding sizes leading to the best validation results are marked as bold.

Besides, we train ComplEx on ICEWS21 for TKG forecasting. We use the implementation provided in the repository of TComplEx. Since ComplEx is not designed for processing temporal information, we transform every quadruple  $(s, r, o, t)$  into a corresponding triplet  $(s, r, o)$ . We do not remove the repeated triplet. For example, if  $(s, r, o, t_1)$  and  $(s, r, o, t_2)$  both exist in the training set of ICEWS21, we train ComplEx with two identical triplets  $(s, r, o)$ . This preserves the inductive bias brought by the temporal knowledge base. To achieve a fairer comparison between ComplEx and TComplEx, we set the embedding size of ComplEx to 100 (same as the embedding size of TComplEx).

We report in Table 2 the validation results of the trained TKG models of all three KG reasoning methods on ICEWS21. We observe that TComplEx underperforms ComplEx in TKG forecasting. We attribute this to the excessive noise introduced by TComplEx’s representations of unseen timestamps. Note that TComplEx is a TKG completion method. The validation timestamps are unseen during training, thus causing TComplEx to leverage the untrained timestamp representations during evaluation. ComplEx does not consider temporal information, which enables it to avoid the negative influence of the timestamps unseen in the training set. TANGO is designed for TKG forecasting. It outperforms the other methods greatly. Although TANGO + Tucker performs better than TANGO + ComplEx on ICEWS21, we choose the latter one for forecasting TKGQA since it aligns to our QA scoring function better.

| Metrics         | MRR   | Hits@1 | Hits@3 | Hits@10 |
|-----------------|-------|--------|--------|---------|
| ComplEx         | 0.278 | 0.188  | 0.312  | 0.456   |
| TComplEx        | 0.250 | 0.164  | 0.279  | 0.420   |
| TANGO + Tucker  | 0.402 | 0.327  | 0.431  | 0.546   |
| TANGO + ComplEx | 0.389 | 0.324  | 0.411  | 0.515   |

Table 2: Validation results of KG reasoning models for TKG forecasting on ICEWS21.

## B.2 Baseline Details

We use the library HuggingFace’s Transformers (Wolf et al. 2019) to implement the pre-trained LMs, i.e., BERT and RoBERTa. Following CRONKGQA and TempoQR, we choose DistilBERT (Sanh et al. 2019) as the BERT model used throughout our work to save computational budget. For every natural language input, e.g., a natural language question, we take the output representation of the [CLS] token computed by an LM as its LM encoded representation.

**Pre-trained LM baselines for TKGQA** We provide detailed information of our pre-trained LM baselines. For entity prediction questions, BERT and RoBERTa compute the scores of all entities with a prediction head  $f_{ep}^{lm}$  as

$$es = f_{ep}^{lm}(\mathbf{h}_q). \quad (5)$$

$es$  is a  $|\mathcal{E}|$ -dimensional real valued vector where each element corresponds to the score of an entity.  $\mathbf{h}_q$  is the question representation output by BERT or RoBERTa with a projection to a  $2d$  real space. Note that in FORECASTTKGQA, we further map the  $2d$  real valued vector to a  $d$ -dimensional complex vector. This step does not exist when we implement pre-trained LM baselines. We choose the entity with the highest score as the predicted answer. BERT\_int and RoBERTa\_int compute the scores  $es$  of all entities with a prediction head  $f_{ep}^{lm.int}$  as

$$es = f_{ep}^{lm.int}(\mathbf{h}_s \parallel \mathbf{h}_q \parallel \mathbf{h}_e \parallel \mathbf{h}_{t_q}), \quad (6)$$

where  $\mathbf{h}_s$ ,  $\mathbf{h}_{t_q}$ , and  $\mathbf{h}_o$  denote the TComplEx representations of the question’s subject entity, the question’s timestamp, and the entity  $e$ , respectively. Similarly, BERT\_ext and RoBERTa\_ext compute the scores  $es$  of all entities with a prediction head  $f_{ep}^{lm.ext}$  as

$$es = f_{ep}^{lm.ext}(\mathbf{h}_{(s,t_q)} \parallel \mathbf{h}_q \parallel \mathbf{h}_{(e,t_q)}), \quad (7)$$

where  $\mathbf{h}_{(s,t_q)}$  and  $\mathbf{h}_{(e,t_q)}$  denote the TANGO representations of the question’s subject entity and the entity  $e$ , respectively. Since TANGO and TComplEx representations are complex vectors in  $\mathcal{C}^d$ , we expand them into  $2d$  real valued vectors, where the first half of every real valued vector is the real part of the original vector and the second half is the imaginary part. This applies to all the TKG representations used in pre-trained LM baselines for answering all three types of questions.

For yes-no questions, BERT and RoBERTa compute the scores of *yes* and *no* with a prediction head  $f_{yn}^{lm}$  as

$$yns = f_{yn}^{lm}(\mathbf{h}_q). \quad (8)$$

$yns$  is a 2-dimensional real valued vector where each element corresponds to the score of either *yes* or *no*. BERT<sub>int</sub> and RoBERTa<sub>int</sub> compute the scores of *yes* and *no* with a prediction head  $f_{yn}^{lm\_int}$  as

$$yns = f_{yn}^{lm\_int}(\mathbf{h}_s \parallel \mathbf{h}_q \parallel \mathbf{h}_o \parallel \mathbf{h}_{t_q}). \quad (9)$$

And BERT<sub>ext</sub> and RoBERTa<sub>ext</sub> compute the scores of *yes* and *no* with a prediction head  $f_{yn}^{lm\_ext}$  as

$$yns = f_{yn}^{lm\_ext}(\mathbf{h}_{(s,t_q)} \parallel \mathbf{h}_q \parallel \mathbf{h}_{(o,t_q)}). \quad (10)$$

We choose the one (either *yes* or *no*) with the higher score as the predicted answer.

For every fact reasoning question, BERT and RoBERTa compute the score  $cs(c_i)$  of the choice  $c_i$  as

$$cs(c_i) = f_{fr}^{lm}(\mathbf{h}_q^{c_i}). \quad (11)$$

$\mathbf{h}_q^{c_i}$  is the output of a pre-trained LM when the concatenation of the question  $q$  and the choice  $c_i$  is given as the input.  $f_{fr}^{lm}$  is a layer of neural network for score computation. BERT<sub>int</sub> and RoBERTa<sub>int</sub> compute the score  $cs(c_i)$  of the choice  $c_i$  as

$$cs(c_i) = f_{fr}^{lm\_int}(\mathbf{h}_q^{lm\_int} \parallel \mathbf{h}_{c_i}^{lm\_int}). \quad (12)$$

$\mathbf{h}_q^{lm\_int} = f_q^{int}(\mathbf{h}_{s_q} \parallel \mathbf{h}_{o_q} \parallel \mathbf{h}_{t_q})$ , where  $\mathbf{h}_{s_q}$ ,  $\mathbf{h}_{o_q}$  and  $\mathbf{h}_{t_q}$  denote the TComplEx representations of the question’s subject entity, object entity and timestamp, respectively.  $f_q^{int}$  is a projection layer for the question.  $\mathbf{h}_{c_i}^{lm\_int} = f_c^{int}(\mathbf{h}_{s_i} \parallel \mathbf{h}_{o_i} \parallel \mathbf{h}_{t_i})$ , where  $\mathbf{h}_{s_i}$ ,  $\mathbf{h}_{o_i}$  and  $\mathbf{h}_{t_i}$  denote the TComplEx representations of the choice’s subject entity, object entity and timestamp, respectively.  $f_c^{int}$  is a projection layer for the choices.  $f_{fr\_int}^{lm}$  is a layer of neural network for score computation. Similarly, BERT<sub>ext</sub> and RoBERTa<sub>ext</sub> compute the score  $cs(c_i)$  of the choice  $c_i$  as

$$cs(c_i) = f_{fr}^{lm\_ext}(\mathbf{h}_q^{lm\_ext} \parallel \mathbf{h}_{c_i}^{lm\_ext}). \quad (13)$$

$\mathbf{h}_q^{lm\_ext} = f_q^{ext}(\mathbf{h}_{(s_q,t_q)} \parallel \mathbf{h}_{(o_q,t_q)}^{c_i})$ , where  $\mathbf{h}_{(s_q,t_q)}$  and  $\mathbf{h}_{(o_q,t_q)}^{c_i}$  denote the TANGO representations of the question’s subject entity and object entity, respectively.  $f_q^{ext}$  is a projection layer for the question.  $\mathbf{h}_{c_i}^{lm\_ext} = f_c^{ext}(\mathbf{h}_{(s_i,t_i)} \parallel \mathbf{h}_{(o_i,t_i)}^{c_i})$ , where  $\mathbf{h}_{(s_i,t_i)}$  and  $\mathbf{h}_{(o_i,t_i)}^{c_i}$  denote the TANGO representations of the choice’s subject entity and object entity, respectively.  $f_c^{ext}$  is a projection layer for the choices.  $f_{fr}^{lm\_ext}$  is a layer of neural network for score computation.

**KGQA & TKGQA Baselines** For EmbedKGQA, we use the trained ComplEx representations as its supporting KG information. For CRONKGQA and TempoQR, we use the trained TComplEx representations as their supporting TKG information. We use the EmbedKGQA and CRONKGQA implementation provided in the repository of CRONKGQA. We use the official implementation of TempoQR. Since we annotate the timestamps for every entity prediction question in FORECASTTKGQUESTIONS, we do not implement soft/hard supervision proposed in TempoQR. We skip the soft/hard supervision and keep everything else as same as the original implementation. We implement all the KGQA baselines with their default hyperparameter settings.

### B.3 FORECASTTKGQA

We search the hyperparameters of FORECASTTKGQA following Table 3. For every type of question, we do 60 trials, and let our model run for 50 epochs. We select the trial leading to the best performance on the validation set and take this hyperparameter setting as our best configuration. We train our model five times with different random seeds and report averaged results. The best hyperparameters concerning all three types of questions are shown in Table 4. We also report the model performance on the validation sets in Table 5 and Table 7. We further report the standard deviation of the results on the test sets in Table 6 and Table 8. The GPU memory usage is reported in Table 9. The training time and test time of our model are presented in Table 10 and Table 11. The number of parameters of our model is presented in Table 12.

| Hyperparameter | Search Space            |
|----------------|-------------------------|
| TKG Model      | {Tucker, ComplEx}       |
| Language Model | {DistilBERT, RoBERTa}   |
| Dropout        | {0.2, 0.3, 0.5}         |
| Batch Size     | {32, 64, 128, 256, 512} |

Table 3: FORECASTTKGQA hyperparameter searching strategy.

| Question Type  | EP         | YN         | FR         |
|----------------|------------|------------|------------|
| Hyperparameter |            |            |            |
| TKG Model      | ComplEx    | ComplEx    | ComplEx    |
| Language Model | DistilBERT | DistilBERT | DistilBERT |
| Dropout        | 0.3        | 0.3        | 0.3        |
| Batch Size     | 512        | 256        | 256        |

Table 4: Best hyperparameter setting. EP, YN, FR denote entity prediction, yes-no, fact reasoning questions, respectively.

## C Dataset Details

### C.1 Data Creation Details

**Data Collection and TKG Construction** We construct a TKG ICEWS21 based on the events taken from the official website of the ICEWS weekly event data (Bosch et al. 2015). We take the events from Jan. 1, 2021, to Aug. 31, 2021, and extract TKG facts in the following way. For every ICEWS event, we generate a TKG fact  $(s, r, o, t)$ . We take the content of "Event Date" as the timestamp  $t$  of the TKG fact. We take the contents of "Source Name" and "Target Name" as the subject entity  $s$  and the object entity  $o$  of the TKG fact, respectively. We take the content of "Event Text" as the relation type  $r$  of the fact. We present the dataset statistics of ICEWS21 in Table 13.

| Model         | MRR     |       |       | Hits@1  |       |       | Hits@10 |       |       |
|---------------|---------|-------|-------|---------|-------|-------|---------|-------|-------|
|               | Overall | 1-Hop | 2-Hop | Overall | 1-Hop | 2-Hop | Overall | 1-Hop | 2-Hop |
| FORECASTTKGQA | 0.299   | 0.343 | 0.295 | 0.208   | 0.248 | 0.114 | 0.477   | 0.527 | 0.356 |

Table 5: Experimental results of entity prediction questions on the validation set. Evaluation metrics are MRR and Hits@1/10.

| Model         | MRR     |        |        | Hits@1  |        |        | Hits@10 |        |        |
|---------------|---------|--------|--------|---------|--------|--------|---------|--------|--------|
|               | Overall | 1-Hop  | 2-Hop  | Overall | 1-Hop  | 2-Hop  | Overall | 1-Hop  | 2-Hop  |
| FORECASTTKGQA | 0.0004  | 0.0004 | 0.0009 | 0.0006  | 0.0007 | 0.0007 | 0.0008  | 0.0008 | 0.0018 |

Table 6: Standard deviation of entity prediction question results on the test set.

| Question Type | Accuracy |                |
|---------------|----------|----------------|
|               | Yes-No   | Fact Reasoning |
| FORECASTTKGQA | 0.887    | 0.560          |

Table 7: Experimental results of yes-no and fact reasoning questions on the validation sets. The evaluation metric is accuracy.

| Question Type | Accuracy |                |
|---------------|----------|----------------|
|               | Yes-No   | Fact Reasoning |
| FORECASTTKGQA | 0.0014   | 0.0049         |

Table 8: Standard deviation of yes-no and fact reasoning question results on the test set.

| Question Type | Entity Prediction | Yes-No     | Fact Reasoning |
|---------------|-------------------|------------|----------------|
| Model         | GPU Memory        | GPU Memory | GPU Memory     |
| FORECASTTKGQA | 45,239MB          | 12,241MB   | 22,719MB       |

Table 9: GPU memory usage.

| Question Type | Entity Prediction | Yes-No | Fact Reasoning |
|---------------|-------------------|--------|----------------|
| Model         |                   |        |                |
| FORECASTTKGQA | 63,840            | 3,700  | 5,800          |

Table 10: Training time (second) of FORECASTTKGQA on all types of questions.

| Question Type | Entity Prediction | Yes-No | Fact Reasoning |
|---------------|-------------------|--------|----------------|
| Model         |                   |        |                |
| FORECASTTKGQA | 48                | 33     | 7              |

Table 11: Test time (second) of FORECASTTKGQA on all types of questions.

**Natural Language Template** After we get ICEWS21, we get a TKG with 253 relation types. Every relation type in ICEWS21 is coupled with a CAMEO code (specified in the "CAMEO Code" column of the ICEWS weekly event

| Question Type | Entity Prediction | Yes-No  | Fact Reasoning |
|---------------|-------------------|---------|----------------|
| Model         |                   |         |                |
| FORECASTTKGQA | 234,600           | 234,600 | 354,800        |

Table 12: Number of parameters of FORECASTTKGQA on all types of questions.

| Dataset | $N_{\text{train}}$ | $N_{\text{valid}}$ | $N_{\text{test}}$ | $ \mathcal{E} $ | $ \mathcal{R} $ | $ \mathcal{T} $ |
|---------|--------------------|--------------------|-------------------|-----------------|-----------------|-----------------|
| ICEWS21 | 252,434            | 43,033             | 39,836            | 20,575          | 253             | 243             |

Table 13: ICEWS21 TKG statistics.  $N_{\text{train}}$ ,  $N_{\text{valid}}$ ,  $N_{\text{test}}$  denote the number of TKG facts in  $\mathcal{G}_{\text{train}}$ ,  $\mathcal{G}_{\text{valid}}$ ,  $\mathcal{G}_{\text{test}}$ , respectively.  $|\mathcal{E}|$ ,  $|\mathcal{R}|$ ,  $|\mathcal{T}|$  denote ICEWS21's number of entities, relations, timestamps, respectively.

data). In the official CAMEO codebook, each CAMEO code is explained with examples and detailed descriptions. We use the official CAMEO codebook provided in the ICEWS dataverse for aiding the generation of natural language templates. We create natural language templates for 250 out of 253 relation types for question generation. For example, we create a natural language template *engage in material cooperation with* for the relation type *Engage in material cooperation, not specified below*. Note that three relation types in ICEWS21 are not taken into consideration because either the verb is not suited for a question in the future tense (*Attempt to assassinate*) or there is no clear description for the subject-object-relationship of the relation type in (Boschee et al. 2015) (*Demobilize armed forces* and *Demonstrate military or police power*). We use the generated natural language templates for question generation of all three types of questions. For fact reasoning questions, we also use these templates to generate natural language choices.

## 2-Hop Entity Prediction Question Generation Details

We generate 2-hop questions by utilizing AnyBURL (Meilicke et al. 2020), a rule-based KG reasoning model. We first split ICEWS21 into TKG snapshots, where each snapshot  $\mathcal{G}_{t_i} = \{(s, r, o, t) \in \mathcal{G} | t = t_i\}$  contains all the TKG facts happening at the same timestamp. We treat every TKG snapshot as a non-temporal KG and train an AnyBURL model with the KG completion task on each TKG snapshot for rule extraction (KG completion aims to predict the missing entity

from every query  $(s, r, ?)$ ). Since AnyBURL is a KG reasoning method that cannot process temporal information, we transform every quadruple  $(s, r, o, t)$  into a corresponding triplet  $(s, r, o)$ . For each TKG snapshot, we keep the 2-hop rules with a confidence higher than 0.5 extracted by AnyBURL, and take them as the drafts of our 2-hop questions.

**Fact Reasoning Question Generation Details** We train xERTE (Han et al. 2021) on ICEWS21 for TKG forecasting, and pick out all the link prediction queries  $(s, r, ?, t)$  whose ground-truth missing entities are ranked by xERTE as top 1. We collect the TKG facts corresponding to these queries for question generation. The intuition of this step is that we assume that the better xERTE performs on a link prediction query, the more reasonable the returned prior facts are for explainability. Ranking the ground-truth missing entities as top 1 indicates that xERTE performs very well on these link prediction queries. We wish to use xERTE to generate reasonable fact reasoning questions, therefore, we want it to find reasonable supporting evidence of the TKG facts by returning relevant prior facts. For each collected "top 1" fact, we take the prior facts with the highest contribution score, the lowest contribution score, the median contribution score, and the second highest contribution score as the fact for generating the choices **Answer**, **Negative**, **Median** and **Hard Negative**, respectively. In this way, we generate a large number of question candidates.

After we collect all the question candidates, we have 78,606 questions. We find that there exist a large number of question candidates whose question and **Answer** share the same  $s, r, o$ . For example, the TKG fact of a question candidate is *(Sudan, host, Ramtane Lamamra, 2021-08-01)*, and the TKG fact of its **Answer** is *(Sudan, host, Ramtane Lamamra, 2021-07-29)*. We filter out all the question candidates with this pattern since we think that they are not satisfying our motivation for proposing fact reasoning questions. We wish to generate the questions that require fact reasoning, rather than finding the repeated facts happening at different timestamps. A good example of the questions we want to generate is as follows. For the question whose associated fact is *(Envoy (United States), visit, China, 2021-08-31)*, the associated fact of its **Answer** is *(Envoy (United States), express the intent to meet or negotiate, China, 2021-08-30)*. From human knowledge, **Answer**'s fact serves as a highly possible reason for the fact in the question, and it is also diverse from the question fact. To this end, we have 50,379 question candidates left.

We then ask three graduate students to label the questions. Students are allowed to use their own knowledge and search engines to help labeling. If the students think that a question's **Answer** is not the most contributive to the question, they are asked to label this question as unreasonable, otherwise, they are asked to label it as reasonable. For every question candidate, if it is labeled as unreasonable by two students, we filter it out. As a result, we have 14,656 questions left.

**Question Time Distribution** We provide the distribution of the questions along the time axis of our dataset in Figure 1 and Figure 2. We plot the number of questions at every

timestamp for all three types of questions.

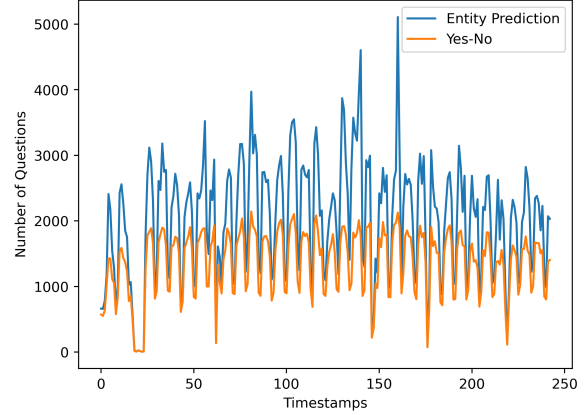

Figure 1: Question distribution of entity prediction and yes-no questions along the time axis.

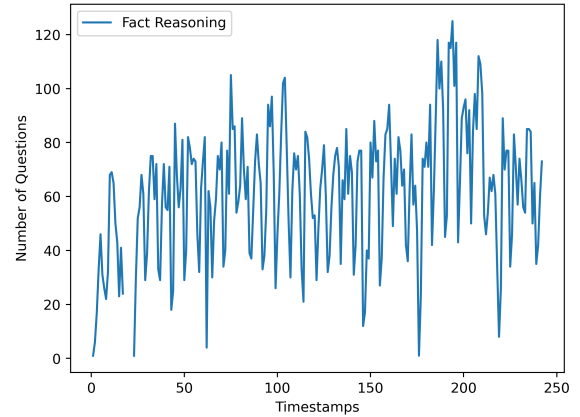

Figure 2: Question distribution of fact reasoning questions along the time axis.

## D Model Structure of FORECASTTKGQA

We present the complete model structure of our model, i.e., FORECASTTKGQA, in Figure 3. We employ TANGO + Complex as our TKG forecasting model. We utilize the learned TKG representations to help boost the model performance on the questions of FORECASTTKGQUESTIONS. We use BERT as the pre-trained LM for encoding natural language information. We design scoring functions of all three types of questions for answer inference.

## E Cross Hop Generalization

We want to study whether the trained model can be generalized between 1-hop and 2-hop entity prediction questions. We train FORECASTTKGQA with only the 1-hop questions

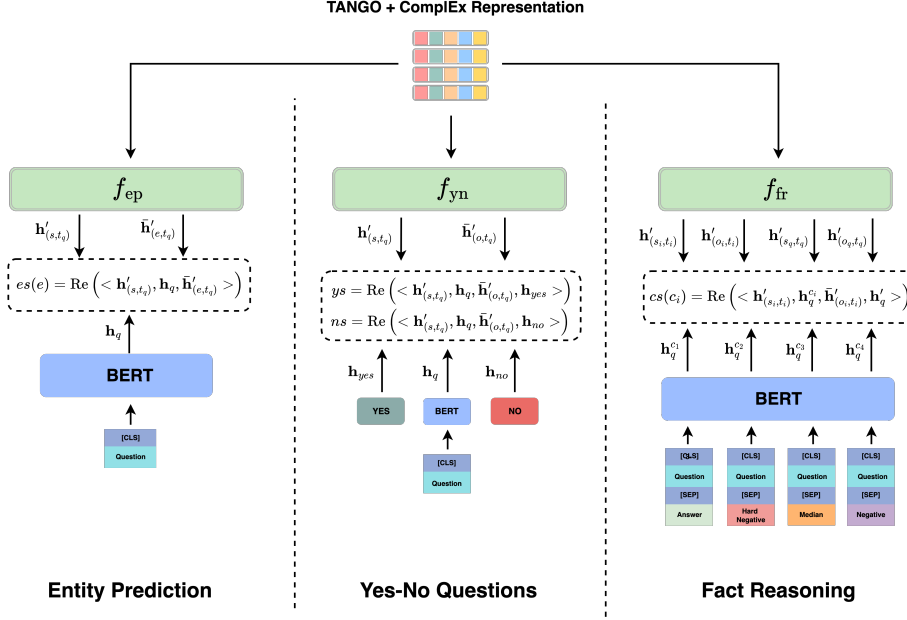

Figure 3: Complete model structure of FORECASTTKGQA.

and evaluate it on the test set of the 2-hop questions. Similarly, we retrain our model with only 2-hop questions and evaluate it on the 1-hop test set. To achieve fair comparison, we randomly sample 1-hop training questions and construct a new 1-hop training set whose size is as same as the complete 2-hop training set, i.e., containing 128,810 questions. In this way, we ensure that when testing on the same test set, our model is trained with the same number of training examples. We observe in Table 14 that our model can preserve about 56% performance when it generalizes from 2-hop to 1-hop questions, and 67% from 1-hop to 2-hop (MRR), showing a strong generalization power.

| Evaluation | 1-Hop |        | 2-Hop |        |
|------------|-------|--------|-------|--------|
|            | MRR   | Hits@1 | MRR   | Hits@1 |
| 1-Hop      | 0.328 | 0.233  | 0.133 | 0.067  |
| 2-Hop      | 0.186 | 0.106  | 0.197 | 0.115  |

Table 14: Cross hop generalization.

## References

- Boschee, E.; Lautenschlager, J.; O’Brien, S.; Shellman, S.; Starz, J.; and Ward, M. 2015. ICEWS Coded Event Data.
- Han, Z.; Chen, P.; Ma, Y.; and Tresp, V. 2021. Explainable Subgraph Reasoning for Forecasting on Temporal Knowledge Graphs. In *9th International Conference on Learning Representations, ICLR 2021, Virtual Event, Austria, May 3-7, 2021*. OpenReview.net.
- Meilicke, C.; Chekol, M. W.; Fink, M.; and Stuckenschmidt, H. 2020. Reinforced Anytime Bottom Up Rule Learning for Knowledge Graph Completion.

- Paszke, A.; Gross, S.; Massa, F.; Lerer, A.; Bradbury, J.; Chanan, G.; Killeen, T.; Lin, Z.; Gimelshein, N.; Antiga, L.; Desmaison, A.; Köpf, A.; Yang, E. Z.; DeVito, Z.; Raison, M.; Tejani, A.; Chilamkurthy, S.; Steiner, B.; Fang, L.; Bai, J.; and Chintala, S. 2019. PyTorch: An Imperative Style, High-Performance Deep Learning Library. In Wallach, H. M.; Larochelle, H.; Beygelzimer, A.; d’Alché-Buc, F.; Fox, E. B.; and Garnett, R., eds., *Advances in Neural Information Processing Systems 32: Annual Conference on Neural Information Processing Systems 2019, NeurIPS 2019, December 8-14, 2019, Vancouver, BC, Canada*, 8024–8035.

- Sanh, V.; Debut, L.; Chaumond, J.; and Wolf, T. 2019. DistilBERT, a distilled version of BERT: smaller, faster, cheaper and lighter. *CoRR*, abs/1910.01108.

- Wolf, T.; Debut, L.; Sanh, V.; Chaumond, J.; Delangue, C.; Moi, A.; Cistac, P.; Rault, T.; Louf, R.; Funtowicz, M.; and Brew, J. 2019. HuggingFace’s Transformers: State-of-the-art Natural Language Processing. *CoRR*, abs/1910.03771.
